# Supplementary material for: A comprehensive and FAIR comparison between MLP and KAN representations for differential equations and operator networks
Source: arXiv:2406.02917 source file (2024-06-05)
Supplement: Supplementary file 1 [file sec_appendix.tex]

\section{Computational details}
